# Supplementary material for: Robust Disentanglement of a Few Factors at a Time
Source: arXiv:2010.13527 source file (2020-10-26)
Supplement: Supplementary file 2 [file appendix_celeba.pdf]

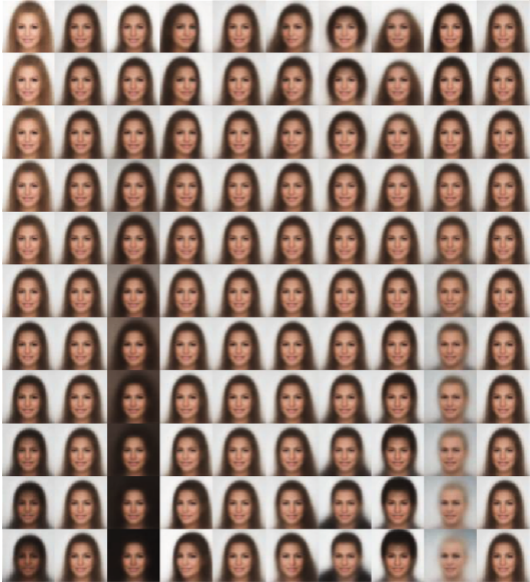

z1

z10
