# Supplementary material for: Robust Disentanglement of a Few Factors at a Time
Source: arXiv:2010.13527 source file (2020-10-26)
Supplement: Supplementary file 3 [file appendix_dsprites.pdf]

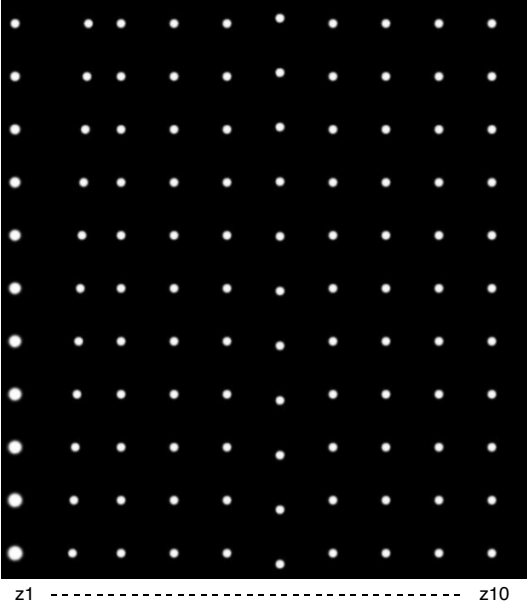

a) supervised *dsprites* traversals

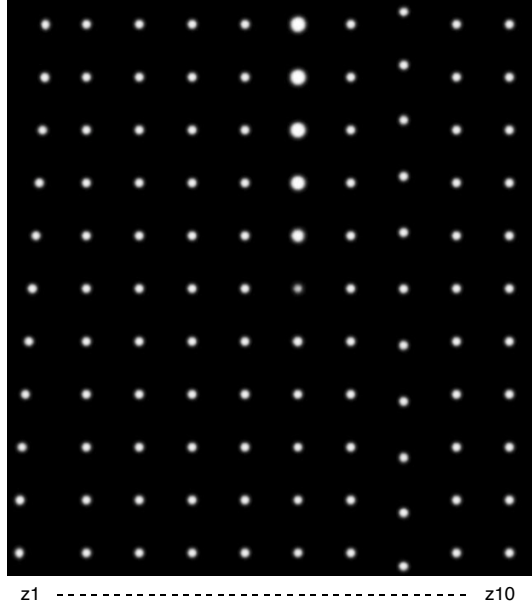

b) unsupervised *dsprites* traversals
